# Supplementary material for: Imaging the Breakdown of Molecular-Frame Dynamics through Rotational Uncoupling
Source: arXiv:1606.02663 ancillary file (2017-07-04)
Supplement: Supplementary file 1 [file supplementary_material.pdf]

# Imaging the breakdown of molecular-frame dynamics through rotational uncoupling - Supplemental Material

**Optical pulse preparation.** A  $\approx 100$  fs 800 nm pulse from a Ti:Sapphire laser was frequency doubled in a BBO crystal cut for Type I second harmonic generation. The residual 800 nm pulse and the 400 nm pulse were then split and recombined in a Mach-Zehnder interferometer using dichroic beam splitters. The delay between the two pulses was controlled by varying the path length of one arm with a motorized translation stage. The intensity of the pulses were set by a separate wave plate in each arm. After recombining, the two pulses co-propagate and pass through a wire grid polarizer before entering a vacuum chamber backfilled with room temperature  $N_2$  gas at a pressure of several  $10^{-8}$  millibar. The pulses are then focused by a spherical mirror with a 15 cm focal length into a velocity map imaging (VMI) spectrometer.

**Extracting the  $4f$  photoelectron angular distribution.** The pump-probe delay was varied between -1 to 30 ps with 700 equally spaced delay points corresponding to  $\sim 45$  fs increments, and the photoelectron momentum distribution was collected at each delay. An example of the raw VMI photoelectron distribution is shown in Fig. S1. The delay points were visited in a randomized order to mitigate any effects caused by long-term drifts of the laser system. The collected photoelectron distribution includes electrons ionized by the 800 nm probe pulse as well as the intense 400 nm pump pulse. In order to eliminate the ionization signal generated by the pump, a background momentum distribution is collected with the 800 nm beam blocked. This distribution is then normalized and subtracted from each pump-probe electron momentum distribution. A moving average of three adjacent delay points is then implemented in order to improve the angular distribution signal.

The photoelectron peak corresponding to the  $4f$  Rydberg manifold is then integrated over in the radial momentum direction. In order to set the limits of integration, we first perform an inverse Abel transform of the raw photoelectron distribution using a polar onion peeling algorithm [1] to get the undistorted angle-integrated momentum distribution, shown in Fig. S2(a). The upper and lower limits of integration are then chosen at the 20% level of the maximum amplitude of the  $4f$  photoelectron peak in the angle-integrated, Abel-inverted momentum distribution. Taking these limits, we then integrate over this region in the raw momentum distribution as depicted in Fig. S2(b). By restricting

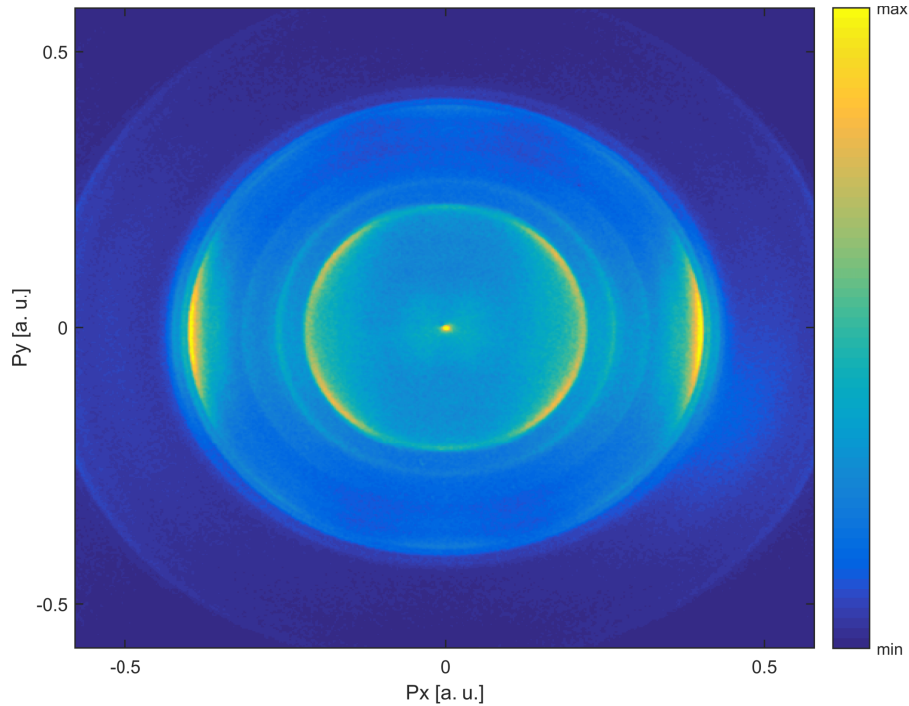

FIG. S1. Raw VMI photoelectron momentum distribution. The innermost bright ring corresponds to single photon ionization of the  $4f$  Rydberg state.

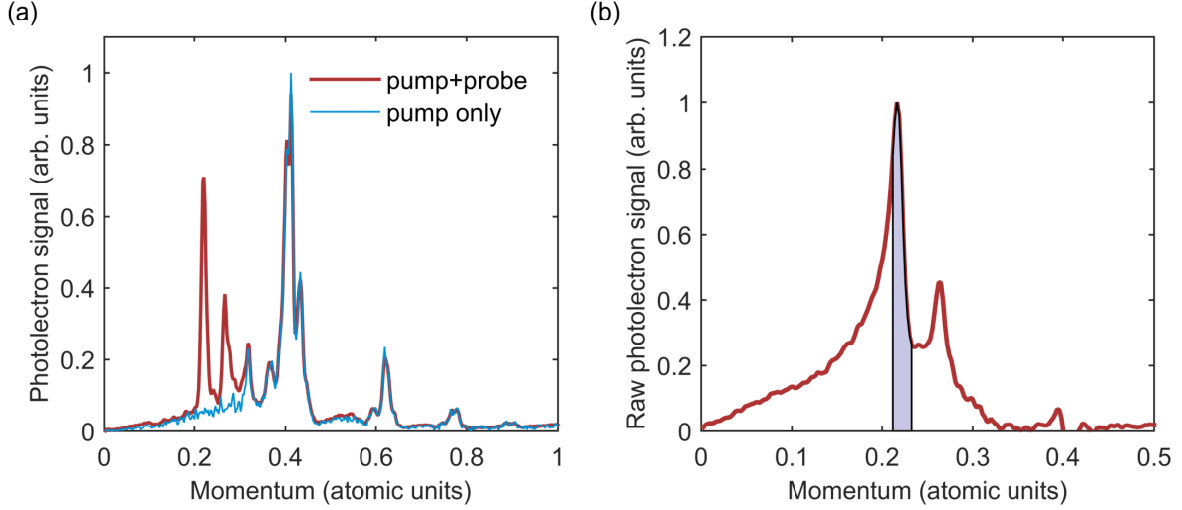

FIG. S2. (a) The Abel-inverted photoelectron momentum distribution from  $N_2$  comparing the pump only signal with the pump+probe signal. The lowest energy photoelectron peak of the pump+probe signal corresponds to the  $4f$  manifold. (b) The raw photoelectron momentum distribution showing the region of the spectrum (shaded area) that is included in the angular distribution extraction of the  $4f$  photoelectron signal.

the integration to this region we limit distortions of the angular distribution due to the "pancaking" of the momentum distribution perpendicular to the detector in a velocity map imaging spectrometer. We then utilize the four-fold symmetry of the system, summing the four angular quadrants together before fitting the angular distribution to a sum of even-ordered Legendre polynomials (Eq. (3) in the main text) using a least-squares method.

**Fourier transform of the time-dependent PAD** The discrete Fourier transforms of the measured and modeled  $\beta_2$  parameter is taken after applying a periodic Hamming window. The signal used in the Fourier transform spans from 300 fs to 30 ps, in order to eliminate transient nonlinear effects when the pump and probe pulses are overlapped in time.

#### Energy levels of the $4f$ manifold in $N_2$

In Fig. S3, the energies of the  $4f$  manifold states as a function of rotational number are plotted with the spectator ion-core rotational energy  $BR(R+1)$  subtracted from the total. The energies are computed from the Hamiltonian

$$H = \hat{H}_{ev} + B\hat{R}^2, \quad (1)$$

where  $\hat{H}_{ev} = -\frac{1}{2(n-\mu_\Lambda)^2}$  is measured relative to the vibrational ground state ionization potential,  $n$  is the principal quantum number, and the quantum defect values  $\delta_\Lambda$  are taken from Ref. [2]. The energies of the Rydberg manifold states, denoted by their Hund's case (d) quantum label  $\mathcal{L} = J - R$ , approach asymptotic values in the limit of large rotations. The quantum label  $\mathcal{L}$  can be interpreted as the projection of the electron orbital angular momentum onto the *rotational* axis [3].

**$l$ -uncoupling Hamiltonian matrix elements.** The rotational-electronic Hamiltonian in Eq. (1) of the main text may be written in terms of angular momentum operators referred to the molecular frame [4]:

$$\begin{aligned} \hat{H} &= \hat{H}_{ev} + B\hat{R}^2 = \hat{H}_{ev} + B[(\hat{J}_x - \hat{l}_x)^2 + (\hat{J}_y - \hat{l}_y)^2] \\ &= \hat{H}_{ev} + B[(\hat{J} - \hat{J}_z)^2 + (\hat{l} - \hat{l}_z)^2 - (\hat{J}_+ \hat{l}_- + \hat{J}_- \hat{l}_+)], \end{aligned} \quad (2)$$

where  $\hat{J}$  is the total angular momentum  $\hat{l}$  is the Rydberg electron orbital angular momentum,  $\hat{J}_\pm, \hat{l}_\pm$  are raising and lowering operators, and the coordinates are referred to the molecular frame with the internuclear axis along the  $z$ -axis. We ignore electron spin in this treatment, since we are concerned with singlet states of  $N_2$ .

The matrix elements of the Hamiltonian are then easily calculated in a Hund's case (b) basis if an integer value of the electron orbital angular momentum is assumed, which is a very good approximation for non-penetrating, high  $l$  molecular Rydberg states. The matrix elements of the angular momentum operators referred to the molecular frame are calculated analogously to lab frame operators, with the exception of the  $\hat{J}_\pm$  operators, which exhibit an anomalous sign [4]:

$$\langle J, (\Lambda + 1) | J_\pm | J, \Lambda \rangle = \sqrt{(J \pm \Lambda)(J \mp \Lambda + 1)}. \quad (3)$$

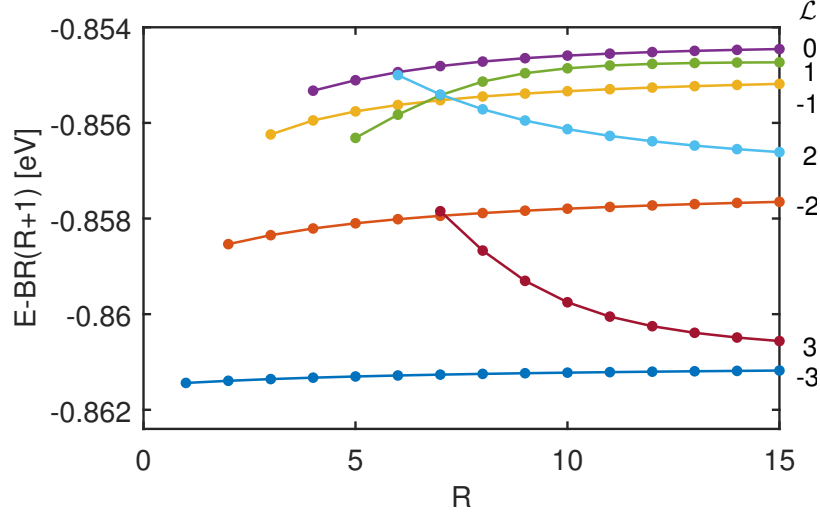

FIG. S3. Energies of the  $4f$  Rydberg manifold in  $N_2$ . The energies of the substates are plotted as a function of the core rotational number  $R$ , with the spectator rotational energy subtracted. The states are labeled according to the Hund's case (d) value of  $\mathcal{L} = J - R$ .

We obtain an energy submatrix for each value of  $J$ , which we then diagonalize to calculate the field-free dynamics of the  $l$ -uncoupling.

**Retrieving the simulated lab frame angular distributions.** After field-free propagation of the  $l$ -uncoupled wave packet, the molecular wave function is projected from Hund's case (b) basis states  $|J, M, l, \Lambda\rangle$ , onto the completely uncoupled Hund's case (d) states  $|J, M, l, R\rangle$ . This is achieved using the vector coupling relations of the molecular frame referenced angular momenta, taking care of the proper phase conventions [5]:

$$|J, M, l, R\rangle = \sum_{\Lambda} (-1)^{R-J-\Lambda} \langle J, \Lambda; l, -\Lambda | R0 \rangle |J, M, l, \Lambda\rangle, \quad (4)$$

where the prefactor in brackets is a Clebsch-Gordan coefficient. From the case (d) basis, the lab frame decoupled electron and ion-core wave functions may then be obtained by a straightforward application of angular momentum coupling:

$$|l, m_l\rangle |R, m_R\rangle = \sum_{J, M} \langle JM | l, m_l; R, m_R \rangle |J, M, l, R\rangle. \quad (5)$$

**Quasi-classical  $l$ -uncoupling demonstration.** For the visualization in Fig. 1 of the main text, an initial rotational state is prepared as a superposition of  $|J, M\rangle$  states where  $J$  is even valued and  $J = M$  for all states. The Gaussian-weighted distribution is centered at  $|J = 30, M = 30\rangle$  with a full width at half maximum of  $\Delta J = 5$ . This localized rotational wave packet approaches the form of a quasi-classical rotating rigid rotor.

**Simulating the multiphoton excitation and photoionization.** Dipole matrix elements are calculated in the single active electron approximation, modeling the  $N_2$  ground state  $\sigma_g$  orbital as an equal superposition of  $s$  and  $d$  partial waves. The rotational  $|JM\rangle$  states are initially populated with a thermal distribution corresponding to a temperature of 295 K for  $N_2$ . We include up to a maximum rotational state of  $J = 20$ . The angular factors of the dipole matrix elements are then calculated exactly, rigorously preserving all selection rules. The direction cosine matrix elements are evaluated with the use of tabulated values [4]. The radial factors are approximated with a propensity term that favors  $l \rightarrow l + 1$  over  $l \rightarrow l - 1$  transitions by a factor of 2. The final photoionization step is calculated after projection of the molecular wave function onto the decoupled  $|l, m_l\rangle |R, m_R\rangle$  basis. In evaluating the dipole matrix elements between the  $4f$  and continuum states, we use hydrogenic radial wave functions, which provide a good approximation for these high  $l$  states due to their small quantum defects.

- [2] K. P. Huber, C. Jungen, K. Yoshino, K. Ito, and G. Stark, *The Journal of Chemical Physics* **100**, 7957 (1994).
- [3] H. Lefebvre-Brion and R. W. Field, in *The Spectra and Dynamics of Diatomic Molecules* (Academic Press, San Diego, 2004) pp. 87–231.
- [4] J. Hougen, *National Bureau of Standards Monograph 115* (U.S. Government Printing Office, 1970).
- [5] J. M. Brown and B. J. Howard, *Molecular Physics* **31**, 1517 (1976).
